# Supplementary material for: Sample Efficient Actor-Critic with Experience Replay
Source: arXiv:1611.01224 source file (2017-07-10)
Supplement: Supplementary file 1 [file appendix.tex]

%!TEX root = ../replay.tex

\section{Further Details on Atari Experiments}
\label{sec:extraDataAtari}
